# Supplementary material for: Electromagnetic moments in the Sn-Gd region determined within nuclear DFT
Source: arXiv:2503.15738 source file (2025-06-03)
Supplement: Supplementary file 1 [file SnGd-SuppMat.pdf]

# Supplemental Material: Nuclear electromagnetic moments in the Sn-Gd region determined within the nuclear DFT

**H Wibowo**[1], **B C Backes**[1], **J Dobaczewski**[1,2], **R P de Groote**[3,4], **A Nagpal**[1], **A Sánchez-Fernández**[1,5,6], **X Sun**[1], **J L Wood**[7]

[1] School of Physics, Engineering and Technology, University of York, Heslington, York YO10 5DD, United Kingdom

[2] Institute of Theoretical Physics, Faculty of Physics, University of Warsaw, ul. Pasteura 5, PL-02-093 Warsaw, Poland

[3] Accelerator Laboratory, Department of Physics, University of Jyväskylä, PB 35(YFL) FIN-40351 Jyväskylä, Finland

[4] KU Leuven, Instituut voor Kern-en Stralingsfysica, B-3001 Leuven, Belgium

[5] Institut d'Astronomie et d'Astrophysique, Université Libre de Bruxelles, Brussels, Belgium

[6] Brussels Laboratory of the Universe - BLU-ULB

[7] School of Physics, Georgia Institute of Technology, Atlanta, Georgia 30332-0430, USA

E-mail: herlik.wibowo@york.ac.uk

**Abstract.** Within the nuclear DFT framework, employing the Skyrme UNEDF1 functional and incorporating pairing correlations, we determined the spectroscopic electric quadrupole and magnetic dipole moments of the $\nu 11/2^-$ and $\pi 7/2^+$ configurations in heavy, deformed, open-shell odd nuclei with $50 \leq Z \leq 64$. The notions of self-consistent shape and spin polarisations due to odd nucleons, which are responsible for generating total electric quadrupole and magnetic dipole moments, were transformed into detailed computational procedures. The alignment of intrinsic angular momentum along the axis of axial symmetry, necessitating signature and time-reversal symmetry breaking, followed by the restoration of rotational symmetry, proved to be essential components of the method. In contrast, the restoration of particle number symmetry yields modifications of only about 1%. With the isovector spin-spin terms of the functional previously

adjusted in near doubly magic nuclei across the mass chart, the calculations were parameter-free. Effective charges and $g$-factors were not employed. A reasonably good agreement was achieved between the calculated and measured electric quadrupole moments. A similarly fair description of the magnetic dipole moments was obtained for the intruder configurations $\nu 11/2^-$ alongside a poor description of those for $\pi 7/2^+$.

Submitted to: *J. Phys. G: Nucl. Phys.*

In the Supplemental material, we list the results obtained in this study as tables of numerical data.

**Table 1.** Calculated spectroscopic quadrupole moments $Q$ (in barns) of the $\nu 11/2^-$ configurations in odd-$N$ nuclei. Entries marked with superscripts $u$ represent global minima in cases where the prolate and oblate tags resulted in identical solutions. Entries marked with superscripts $p$ and $o$ represent global minima in cases where the prolate and oblate tags resulted in different solutions. In these latter cases, superscripts $p$ ($o$) represent the solutions where prolate (oblate) tags resulted in lower energies than the oblate (prolate) tags.

| | Sn | Te | Xe | Ba | Ce | Nd | Sm | Gd |
|---|---|---|---|---|---|---|---|---|
| $N$-$Z$ | Z=50 | Z=52 | Z=54 | Z=56 | Z=58 | Z=60 | Z=62 | Z=64 |
| 1 | $-0.249^u$ | $-0.837^u$ | $-1.534^o$ | $-2.041^o$ | $-2.506^o$ | $-2.802^o$ | $-2.805^o$ | $-2.768^o$ |
| 3 | $-0.386^u$ | $-1.107^u$ | $-1.718^o$ | $-2.059^{o,a}$ | $-2.429^o$ | $-2.667^o$ | $-2.666^o$ | $-2.722^o$ |
| 5 | $-0.507^u$ | $-1.321^o$ | $-1.836^o$ | $-2.076^o$ | $-2.325^o$ | $-2.501^o$ | $-2.594^o$ | $3.924^p$ |
| 7 | $-0.683^u$ | $-1.418^o$ | $-1.746^o$ | $-1.987^o$ | $-2.223^o$ | $-2.420^o$ | $3.747^p$ | $3.798^p$ |
| 9 | $-0.816^u$ | $-1.371^o$ | $-1.672^o$ | $-1.925^o$ | $-2.177^o$ | $3.475^p$ | $3.504^p$ | $3.395^p$ |
| 11 | $-0.842^u$ | $-1.309^o$ | $-1.628^o$ | $-1.901^o$ | $-2.136^o$ | $3.110^p$ | $3.028^p$ | $2.770^p$ |
| 13 | $-0.786^u$ | $-1.248^u$ | $-1.594^o$ | $-1.817^o$ | $2.646^p$ | $2.650^p$ | $2.421^p$ | $1.585^u$ |
| 15 | $-0.653^u$ | $-1.132^u$ | $-1.473^o$ | $2.221^p$ | $2.306^p$ | $2.112^p$ | $1.627^u$ | $0.708^u$ |
| 17 | $-0.472^u$ | $-0.957^u$ | $-1.253^o$ | $2.012^p$ | $1.896^p$ | $1.593^u$ | $0.841^u$ | $0.546^u$ |
| 19 | $-0.300^u$ | $-0.745^u$ | $1.518^p$ | $1.697^p$ | $1.508^u$ | $1.017^u$ | $0.588^u$ | $1.292^u$ |
| 21 | $-0.170^u$ | $-0.391^u$ | $1.267^p$ | $1.353^u$ | $1.065^u$ | $0.657^u$ | $1.361^u$ | $2.522^u$ |
| 23 | $-0.079^u$ | $-0.018^u$ | $0.969^u$ | $0.959^u$ | $0.687^u$ | $1.437^u$ | $2.304^u$ | $3.231^u$ |
| 25 | $-0.007^u$ | $0.186^u$ | $0.658^u$ | $0.629^u$ | $1.451^u$ | $2.064^u$ | $2.974^u$ | $3.846^p$ |
| 27 | $0.059^u$ | $0.297^u$ | $0.493^u$ | $1.384^u$ | $1.924^u$ | $2.646^u$ | $3.769^p$ | $4.320^p$ |
| 29 | $0.124^u$ | $0.329^u$ | $1.176^u$ | $1.815^u$ | $2.345^u$ | $3.666^p$ | $4.251^p$ | $4.568^p$ |
| 31 | $0.176^u$ | $0.745^u$ | $1.544^u$ | $2.129^u$ | $3.002^p$ | $4.215^p$ | $4.467^p$ | $4.744^p$ |
| 33 | $0.262^u$ | $1.125^u$ | $1.811^u$ | $2.346^p$ | $3.526^p$ | $4.359^p$ | $4.645^{p,a}$ | $4.827^p$ |
| 35 | $0.339^u$ | $1.435^u$ | $1.998^u$ | $2.585^p$ | $3.773^p$ | $4.490^p$ | $4.716^p$ | $4.885^p$ |
| 37 | $0.374^u$ | $1.610^u$ | $2.195^p$ | $3.045^p$ | $3.974^p$ | $4.555^p$ | $4.765^p$ | $4.932^p$ |
| 39 | $0.377^u$ | $1.790^u$ | $2.462^p$ | $3.448^p$ | $4.147^p$ | $4.603^p$ | $4.850^p$ | $4.972^p$ |

$^o$ oblate tag solution.
$^p$ prolate tag solution.
$^u$ unique solution.
$^a$ interpolated result.

**Table 2.** Calculated spectroscopic magnetic dipole moments $\mu$ of the $\nu 11/2^-$ configurations in odd-$N$ nuclei (in $\mu_N$). Superscripts shown in Table 1 pertain also to all entries of this Table.

| | Sn | Te | Xe | Ba | Ce | Nd | Sm | Gd |
|---|---|---|---|---|---|---|---|---|
| $N$-$Z$ | Z=50 | Z=52 | Z=54 | Z=56 | Z=58 | Z=60 | Z=62 | Z=64 |
| 1 | −1.243 | −0.939 | −0.719 | −0.712 | −0.767 | −0.755 | −0.857 | −0.928 |
| 3 | −1.171 | −0.811 | −0.732 | −0.766 | −0.800 | −0.819 | −0.912 | −0.942 |
| 5 | −1.095 | −0.762 | −0.782 | −0.819 | −0.845 | −0.891 | −0.936 | −0.885 |
| 7 | −0.986 | −0.779 | −0.821 | −0.858 | −0.896 | −0.925 | −0.884 | −0.888 |
| 9 | −0.920 | −0.830 | −0.858 | −0.895 | −0.921 | −0.874 | −0.906 | −0.900 |
| 11 | −0.942 | −0.885 | −0.890 | −0.913 | −0.909 | −0.925 | −0.941 | −0.909 |
| 13 | −1.016 | −0.936 | −0.910 | −0.923 | −0.945 | −0.970 | −0.958 | −1.080 |
| 15 | −1.128 | −0.997 | −0.944 | −0.934 | −0.978 | −0.994 | −1.056 | −1.305 |
| 17 | −1.256 | −1.084 | −1.021 | −0.953 | −1.007 | −1.046 | −1.255 | −1.286 |
| 19 | −1.351 | −1.193 | −0.991 | −0.999 | −1.054 | −1.180 | −1.274 | −1.078 |
| 21 | −1.397 | −1.363 | −1.051 | −1.068 | −1.149 | −1.246 | −1.044 | −0.894 |
| 23 | −1.406 | −1.431 | −1.148 | −1.167 | −1.224 | −1.006 | −0.919 | −0.842 |
| 25 | −1.392 | −1.386 | −1.244 | −1.226 | −0.991 | −0.938 | −0.877 | −0.840 |
| 27 | −1.356 | −1.320 | −1.242 | −0.987 | −0.938 | −0.914 | −0.849 | −0.869 |
| 29 | −1.308 | −1.253 | −1.002 | −0.917 | −0.931 | −0.838 | −0.874 | −0.891 |
| 31 | −1.244 | −1.100 | −0.928 | −0.908 | −0.888 | −0.814 | −0.899 | −0.889 |
| 33 | −1.208 | −0.942 | −0.923 | −0.921 | −0.893 | −0.844 | −0.902 | −0.869 |
| 35 | −1.171 | −0.845 | −0.931 | −0.940 | −0.927 | −0.851 | −0.880 | −0.845 |
| 37 | −1.146 | −0.825 | −0.944 | −0.966 | −0.925 | −0.827 | −0.852 | −0.849 |
| 39 | −1.138 | −0.860 | −0.960 | −0.963 | −0.902 | −0.814 | −0.858 | −0.873 |

**Table 3.** Same as in Table 1 but for the $\pi 7/2^+$ configurations in odd-$Z$ nuclei.

| | Sb | I | Cs | La | Pr | Pm | Eu |
|---|---|---|---|---|---|---|---|
| $N$-$Z$ | Z=51 | Z=53 | Z=55 | Z=57 | Z=59 | Z=61 | Z=63 |
| −1 | $-0.294^u$ | $-0.660^u$ | $-1.087^o$ | $-1.542^o$ | $-2.019^o$ | $3.117^p$ | $3.265^p$ |
| 1 | $-0.416^u$ | $-0.866^o$ | $-1.270^o$ | $-1.720^o$ | $-2.186^o$ | $3.094^p$ | $3.213^p$ |
| 3 | $-0.549^u$ | $-1.009^o$ | $-1.411^o$ | $-1.891^o$ | $-2.168^o$ | $3.055^p$ | $3.090^p$ |
| 5 | $-0.682^u$ | $-1.103^o$ | $-1.517^o$ | $-1.858^o$ | $-2.106^o$ | $2.927^p$ | $2.938^p$ |
| 7 | $-0.775^u$ | $-1.158^o$ | $-1.513^o$ | $-1.796^o$ | $-2.010^o$ | $2.721^p$ | $2.726^p$ |
| 9 | $-0.833^u$ | $-1.185^{o,a}$ | $-1.482^o$ | $-1.742^o$ | $-1.950^o$ | $2.413^p$ | $2.326^p$ |
| 11 | $-0.869^u$ | $-1.200^u$ | $-1.463^o$ | $-1.719^o$ | $-1.952^o$ | $1.997^p$ | $1.897^p$ |
| 13 | $-0.889^u$ | $-1.206^u$ | $-1.451^o$ | $-1.703^o$ | $1.694^p$ | $1.615^p$ | $1.542^p$ |
| 15 | $-0.873^u$ | $-1.183^u$ | $-1.384^o$ | $-1.526^o$ | $1.420^p$ | $1.328^p$ | $1.164^u$ |
| 17 | $-0.798^u$ | $-1.100^u$ | $-1.202^{o,a}$ | $1.249^p$ | $1.187^p$ | $1.056^u$ | $0.736^u$ |
| 19 | $-0.704^u$ | $-0.977^u$ | $-0.996^o$ | $1.021^p$ | $0.935^o$ | $0.694^u$ | $0.312^u$ |
| 21 | $-0.607^u$ | $-0.834^u$ | $-0.763^o$ | $0.723^u$ | $0.563^u$ | $0.273^u$ | $0.696^u$ |
| 23 | $-0.502^u$ | $-0.610^u$ | $-0.351^u$ | $0.190^u$ | $0.195^u$ | $0.683^u$ | $1.275^u$ |
| 25 | $-0.415^u$ | $-0.383^u$ | $-0.130^u$ | $0.078^u$ | $0.639^u$ | $1.121^u$ | $1.822^p$ |
| 27 | $-0.355^u$ | $-0.251^u$ | $-0.048^u$ | $0.484^u$ | $1.066^u$ | $1.537^p$ | $2.417^p$ |
| 29 | $-0.308^u$ | $-0.164^u$ | $-0.155^u$ | $0.979^u$ | $1.367^p$ | $2.072^p$ | $2.876^p$ |
| 31 | $-0.262^u$ | $-0.287^u$ | $0.719^p$ | $1.262^p$ | $1.601^p$ | $2.855^p$ | $3.062^p$ |
| 33 | $-0.329^u$ | $-0.423^u$ | $0.981^p$ | $1.434^p$ | $2.259^p$ | $3.043^p$ | $3.173^p$ |
| 35 | $-0.377^u$ | $-0.566^u$ | $1.128^p$ | $1.576^p$ | $2.484^p$ | $3.108^{p,a}$ | $3.234^p$ |
| 37 | $-0.419^u$ | $-0.754^u$ | $1.242^p$ | $1.719^p$ | $2.574^p$ | $3.172^p$ | $3.264^p$ |
| 39 | $-0.466^u$ | $-0.949^{o,a}$ | $-1.414^o$ | $1.861^p$ | $2.632^p$ | $3.171^p$ | $3.255^p$ |

$^o$ oblate tag solution.

$^p$ prolate tag solution.

$^u$ unique solution.

$^a$ interpolated result.

**Table 4.** Same as in Table 2 but for the $\pi 7/2^+$ configurations in odd-$Z$ nuclei.

| | Sb | I | Cs | La | Pr | Pm | Eu |
|---|---|---|---|---|---|---|---|
| $N$-$Z$ | Z=51 | Z=53 | Z=55 | Z=57 | Z=59 | Z=61 | Z=63 |
| −1 | 2.272 | 2.402 | 2.553 | 2.716 | 2.916 | 1.925 | 1.861 |
| 1 | 2.308 | 2.517 | 2.643 | 2.808 | 2.991 | 1.934 | 1.860 |
| 3 | 2.365 | 2.593 | 2.711 | 2.895 | 2.995 | 1.917 | 1.860 |
| 5 | 2.433 | 2.635 | 2.764 | 2.872 | 2.928 | 1.898 | 1.848 |
| 7 | 2.478 | 2.652 | 2.744 | 2.806 | 2.818 | 1.860 | 1.830 |
| 9 | 2.497 | 2.647 | 2.695 | 2.733 | 2.736 | 1.833 | 1.814 |
| 11 | 2.498 | 2.630 | 2.650 | 2.686 | 2.726 | 1.794 | 1.830 |
| 13 | 2.489 | 2.610 | 2.621 | 2.669 | 1.815 | 1.819 | 1.861 |
| 15 | 2.464 | 2.587 | 2.580 | 2.563 | 1.848 | 1.865 | 1.896 |
| 17 | 2.415 | 2.541 | 2.472 | 1.915 | 1.888 | 1.911 | 1.984 |
| 19 | 2.365 | 2.468 | 2.353 | 1.933 | 1.927 | 1.983 | 2.068 |
| 21 | 2.328 | 2.385 | 2.255 | 1.964 | 1.993 | 2.050 | 2.015 |
| 23 | 2.298 | 2.283 | 2.142 | 2.046 | 2.045 | 2.006 | 1.923 |
| 25 | 2.280 | 2.212 | 2.116 | 2.068 | 2.002 | 1.928 | 1.898 |
| 27 | 2.273 | 2.192 | 2.118 | 2.026 | 1.936 | 1.864 | 1.922 |
| 29 | 2.276 | 2.191 | 2.140 | 1.969 | 1.876 | 1.881 | 1.900 |
| 31 | 2.284 | 2.216 | 2.030 | 1.928 | 1.842 | 1.937 | 1.865 |
| 33 | 2.297 | 2.254 | 1.987 | 1.899 | 1.880 | 1.923 | 1.854 |
| 35 | 2.314 | 2.314 | 1.950 | 1.869 | 1.857 | 1.917 | 1.853 |
| 37 | 2.332 | 2.413 | 1.922 | 1.837 | 1.840 | 1.910 | 1.850 |
| 39 | 2.349 | 2.527 | 2.754 | 1.806 | 1.828 | 1.893 | 1.833 |
